# Supplementary material for: Infinite-pressure phase diagram of binary mixtures of (non)additive hard disks
Source: arXiv:2003.08889 ancillary file (2020-05-28)
Supplement: Supplementary file 1 [file SI.pdf]

# Supplemental information: Infinite-pressure phase diagram of binary mixtures of (non)additive hard disks

## I. DEFORMATION PATHS

Phases drawn in Fig. 3 of the main text depict the structures at "magic ratios" where they are highly symmetric, with a large number of contacts between the disks. When the size ratio $q$ deviates from those values, structures are deformed, bonds are broken and parts of the symmetry are broken. In Fig. 1-12, we present deformation paths for the phases that appear in the phase diagrams, in which we highlight how the contacts between particles (red lines) are changed upon deformation between different magic size ratios. In some cases, multiple paths are possible, which will have different volumes per particle depending on the exact choice of size ratio and non-additivity parameter.

In Table I, we provide numerical values for the various magic ratios for $\Delta = 0, 0.03, 0.05$ and 0.1. Each crystal structure has several magic ratios associated with its deformation path, as indicated in the associated figure (Fig. 1-12). For example, $q_{T2\_2}$ is the magic ratio for crystal structure T2, with index 2. Note that some magic ratios that carry different labels are actually identical.

All deformations are obtained from Floppy Box Monte Carlo simulations[1]. Some structures that have the same composition $x_S$ can deform continuously one into the other, even if they are given separate names in the main text to conform to the naming scheme of Ref. 2. In such cases, the deformation paths are linked together and each phase corresponds to one portion.

| label | $\Delta = 0$ | $\Delta = 0.03$ | $\Delta = 0.05$ | $\Delta = 0.1$ |
|---|---|---|---|---|
| $q_{T1\_0}$ | 0.155 | 0.190 | 0.215 | 0.283 |
| $q_{T1\_1}$ | 0.281 | 0.308 | 0.327 | 0.376 |
| $q_{T2\_0}$ | 0.101 | 0.124 | 0.140 | 0.183 |
| $q_{T2\_1}$ | 0.216 | 0.220 | 0.224 | 0.235 |
| $q_{T2\_2}$ | 0.349 | 0.335 | 0.326 | 0.304 |
| $q_{T3\_0}$ | 0.082 | 0.101 | 0.115 | 0.152 |
| $q_{T3\_1}$ | 0.119 | 0.131 | 0.139 | 0.163 |
| $q_{T3\_2}$ | 0.233 | 0.224 | 0.219 | 0.205 |
| $q_{T4\_0}$ | 0.349 | 0.335 | 0.326 | 0.304 |
| $q_{T4\_1}$ | 0.308 | 0.319 | 0.326 | 0.344 |
| $q_{S1\_0}$ | 0.155 | 0.190 | 0.215 | 0.283 |
| $q_{S1\_1}$ | 0.414 | 0.458 | 0.489 | 0.571 |
| $q_{S2\_0}$ | 0.101 | 0.124 | 0.140 | 0.183 |
| $q_{S2\_1}$ | 0.217 | 0.238 | 0.252 | 0.290 |
| $q_{S2\_2}$ | 0.369 | 0.372 | 0.374 | 0.381 |
| $q_{S2\_3}$ | 0.620 | 0.590 | 0.571 | 0.525 |
| $q_{S3\_0}$ | 0.187 | 0.204 | 0.217 | 0.250 |
| $q_{S3\_1}$ | 0.473 | 0.453 | 0.439 | 0.407 |
| $q_{S4\_0}$ | 0.073 | 0.090 | 0.102 | 0.136 |
| $q_{S4\_1}$ | 0.199 | 0.162 | 0.149 | 0.131 |
| $q_{S4\_2}$ | 0.136 | 0.149 | 0.156 | 0.175 |
| $q_{S4\_3}$ | 0.288 | 0.284 | 0.281 | 0.272 |
| $q_{S5\_0}$ | 0.244 | 0.248 | 0.251 | 0.260 |
| $q_{S5\_1}$ | 0.389 | 0.373 | 0.363 | 0.337 |
| $q_{H1\_0}$ | 0.533 | 0.536 | 0.538 | 0.543 |
| $q_{H1\_1}$ | 1 | 0.942 | 0.905 | 0.818 |
| $q_{H2\_0}$ | 0.638 | 0.669 | 0.691 | 0.748 |
| $q_{H3\_0}$ | 0.101 | 0.124 | 0.140 | 0.183 |
| $q_{H3\_1}$ | 0.386 | 0.404 | 0.416 | 0.448 |
| $q_{H3\_2}$ | 1 | 0.942 | 0.905 | 0.818 |
| $q_{H4\_0}$ | 1 | 0.942 | 0.905 | 0.818 |
| $q_{Sh1\_0}$ | 0.101 | 0.124 | 0.140 | 0.183 |
| $q_{Sh1\_1}$ | 0.545 | 0.571 | 0.589 | 0.636 |

TABLE I. "Magic" size ratios where the various crystal structures exactly accomodate a specific set of contacts between neighbors.

## II. SHIELDS-TRIANGLES STRUCTURES

The Sh1 unit cell can be decomposed into a shield-shaped tile and triangular $\text{Hex}_L$ tiles. Those tiles can be combined without volume-per-particle cost for $q \leq q_{Sh\_0}(\delta)$ (see Fig. 11). While these shields and triangles do not allow random tiling of the plane, they can be combined into a family of periodic structures with larger and larger unit cells[3]. In Figure 13 we show the two first members ($n = 1$ and $n = 2$) of an infinite family of periodic structures that exist for a fraction of small disks. In this family, the structure with index $n$ has a composition

$$x_S(n) = \frac{3n(n+1)}{6n(n+1)+1}. \quad (1)$$

In the limit where $n \to \infty$ this converges to $x_S = 1/2$, and the phase becomes identical to the Sh1 phase. However, for small $n$, the composition is slightly smaller, as extra large particles are included at the crossing points of the red lines in Fig. 13. Since this inclusion of $\text{Hex}_L$ tiles comes without volume cost, structures within this family (or coexistences between them) are exactly as stable as the $\text{Hex}_L$-Sh1 coexistence at infinite pressure at their respective compositions. Hence, there is a small region of many competing tilings at compositions between $x_S = 6/13$ and $1/2$ in the phase diagram in Fig. 4 of the main text. At finite pressure, we expect that vibrationnal entropy contribution will favor one of these crystals and simplify this region of the phase diagram.

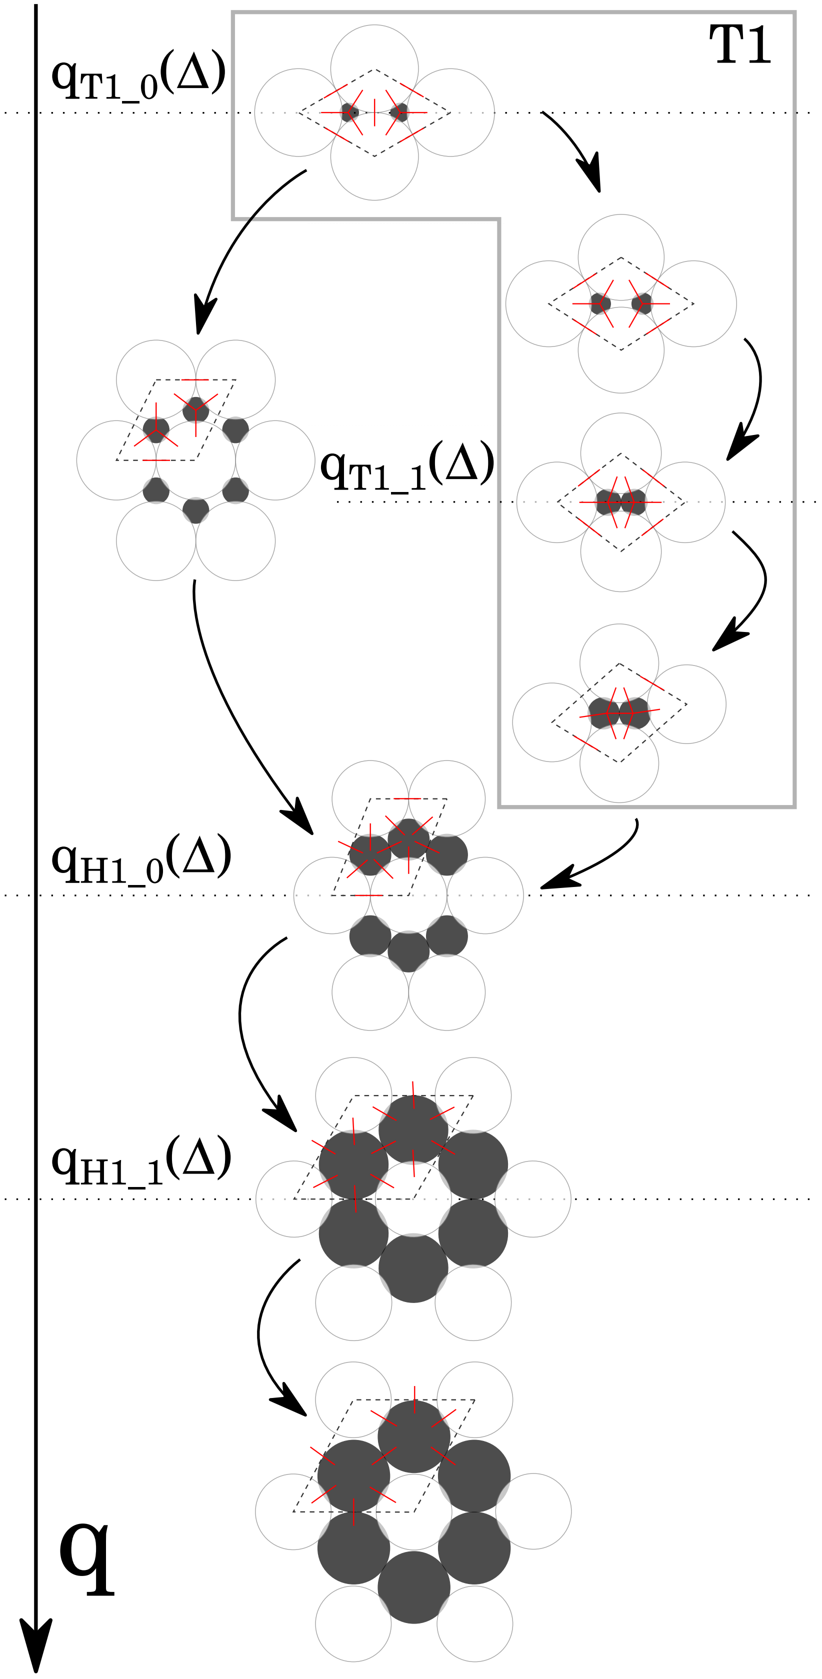


FIG. 1. T1 and H1 deformation paths. Both phase have the same composition and can continuously deform one into the other at $q = q_{H1\_0}(\Delta)$. We call T1 the branch of the path in the grey frame. The other portions are labelled H1.

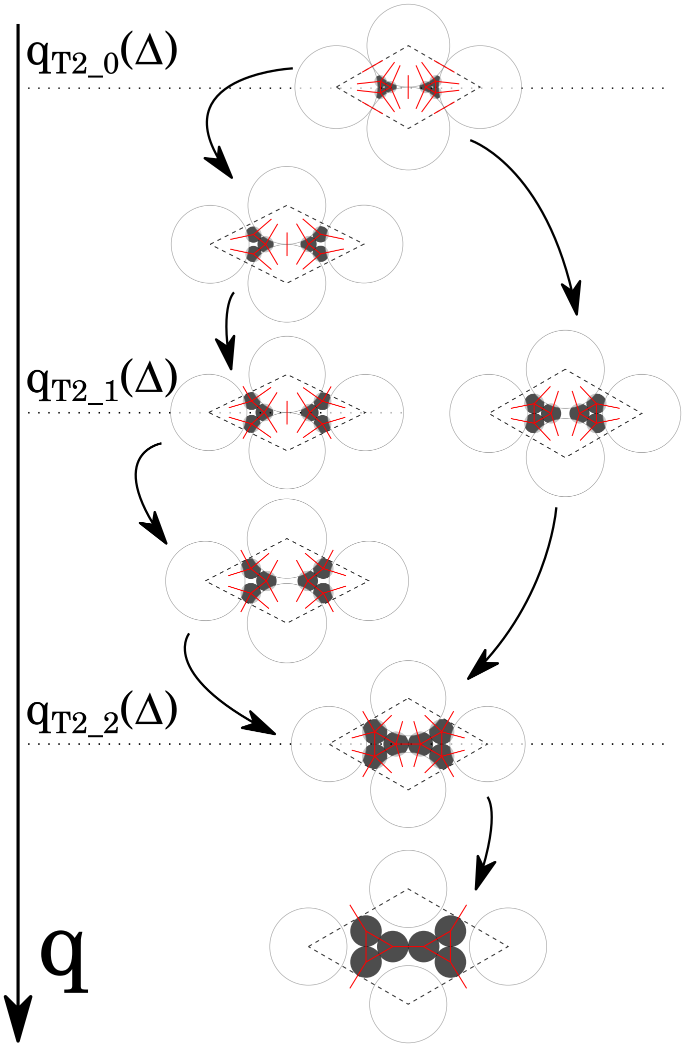


FIG. 2. T2 deformation path. There are two ways to expand the unit cell above $q_{T2\_0}(\Delta)$. The right branch takes over the other in terms of volume per particle at a size ratio between $q_{T2\_0}(\Delta)$ and $q_{T2\_2}(\Delta)$, that does not correspond to a magic ratio. We decide to keep the same name T2 for both branches to lighten the naming scheme.

In our simulations, we only consider periodic crystals with up to 12 disks in the unit cell so the family of structures mentioned above is out of scope. However, we note that the existence of these complex structures suggests that periodic structures with large unit cells may exist elsewhere, when unit cells of coexisting phases can be decomposed into a set of matching tiles that can tile the plane in a variety of ways, even if fully aperiodic tilings are not possible.

## III. CALCULATIONS OF THE VOLUMES PER PARTICLE

Candidate crystal structures are sampled by FBMC simulations for discrete values of the size ratio $q$ and composition $x_S$. To draw the phase diagrams and get the exact range of stability of the different phases, we compute their volume per particle $v$ along the deformation paths. To this end, we identify the disks in contact from the simulations, and write down a set of equations for the position of all the disks in the unit cell. Then, we use the symbolic math library `Sympy`[4] to obtain analytic expressions for the particle positions and the volume per particle of each structure as a function of $q$ and $\Delta$.

In some cases, `Sympy` fails to solve the equation for the magic ratio. We then rely on a numerical solution. In the worst case (S4), we did not find analytical expressions for the position of the particles. For this case, we compute the positions numerically, deduce the volume per particle for a large number of $(q, \Delta)$ points and use 2D linear interpolation to estimate missing values.

Fig. 14 displays the packing fraction of the pure phases that appear in the additive phase diagram ($\Delta = 0$) of the main text. Note that the best packing phase in these diagrams is not necessarily the stable phase, because a

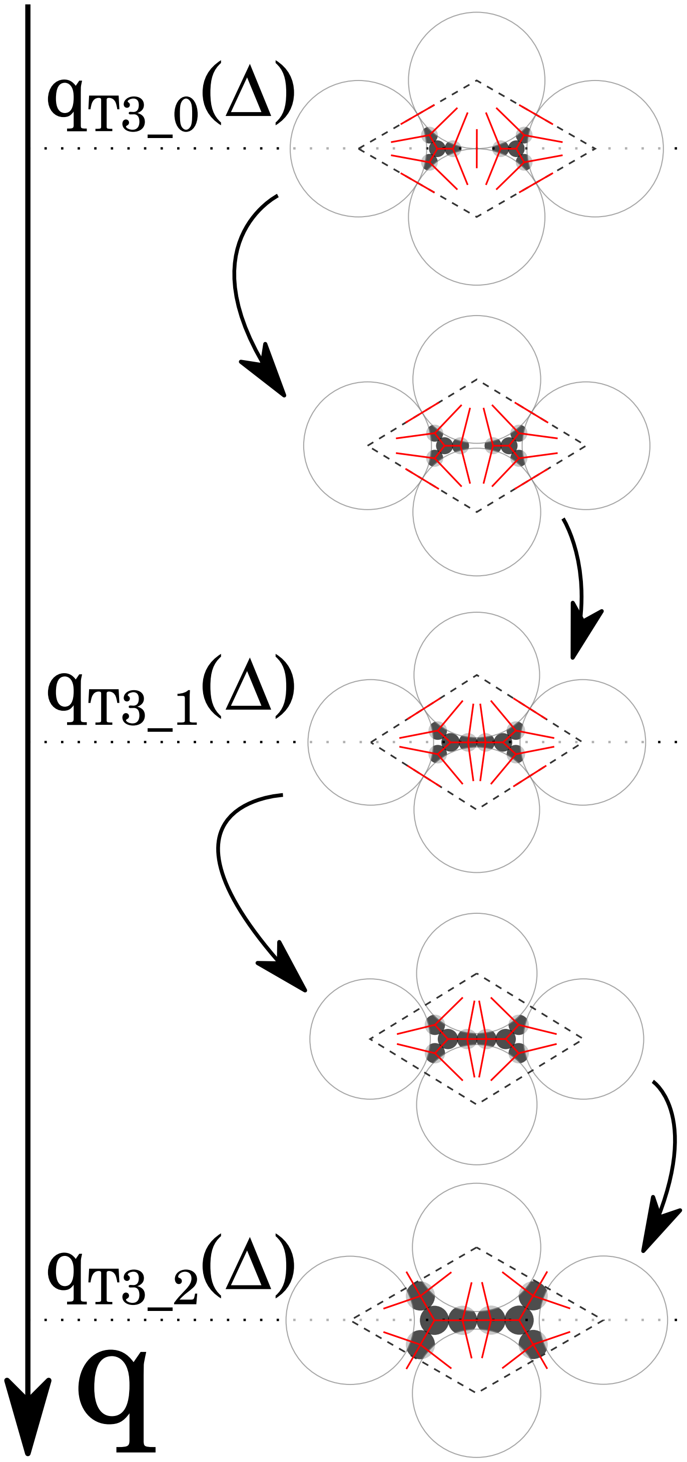


FIG. 3. T3 deformation path.

coexistence of two phases (not shown in the graph), could pack better at this composition.

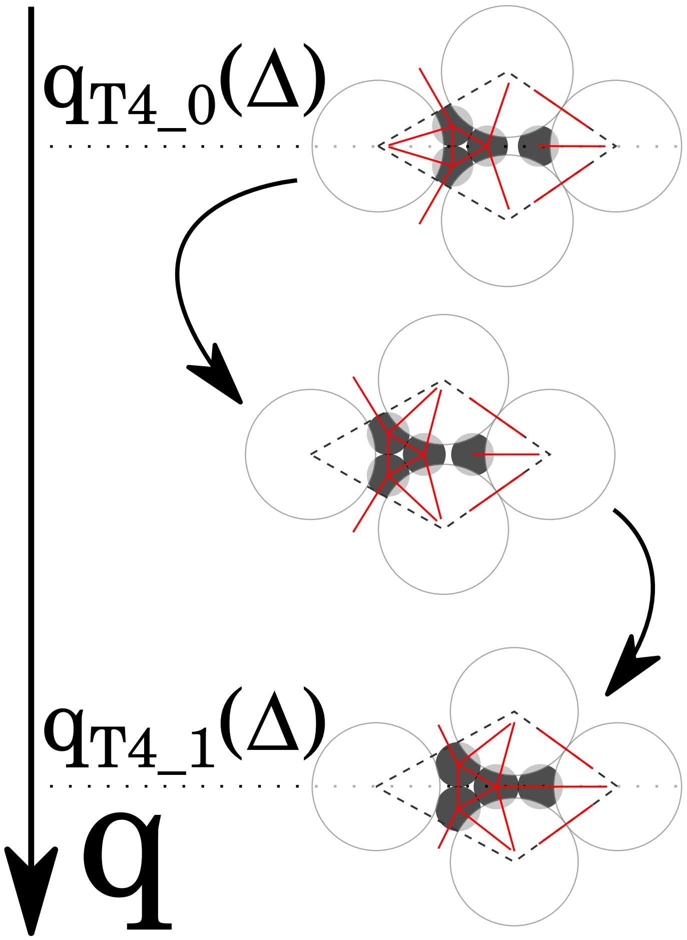


FIG. 4. T4 deformation path.

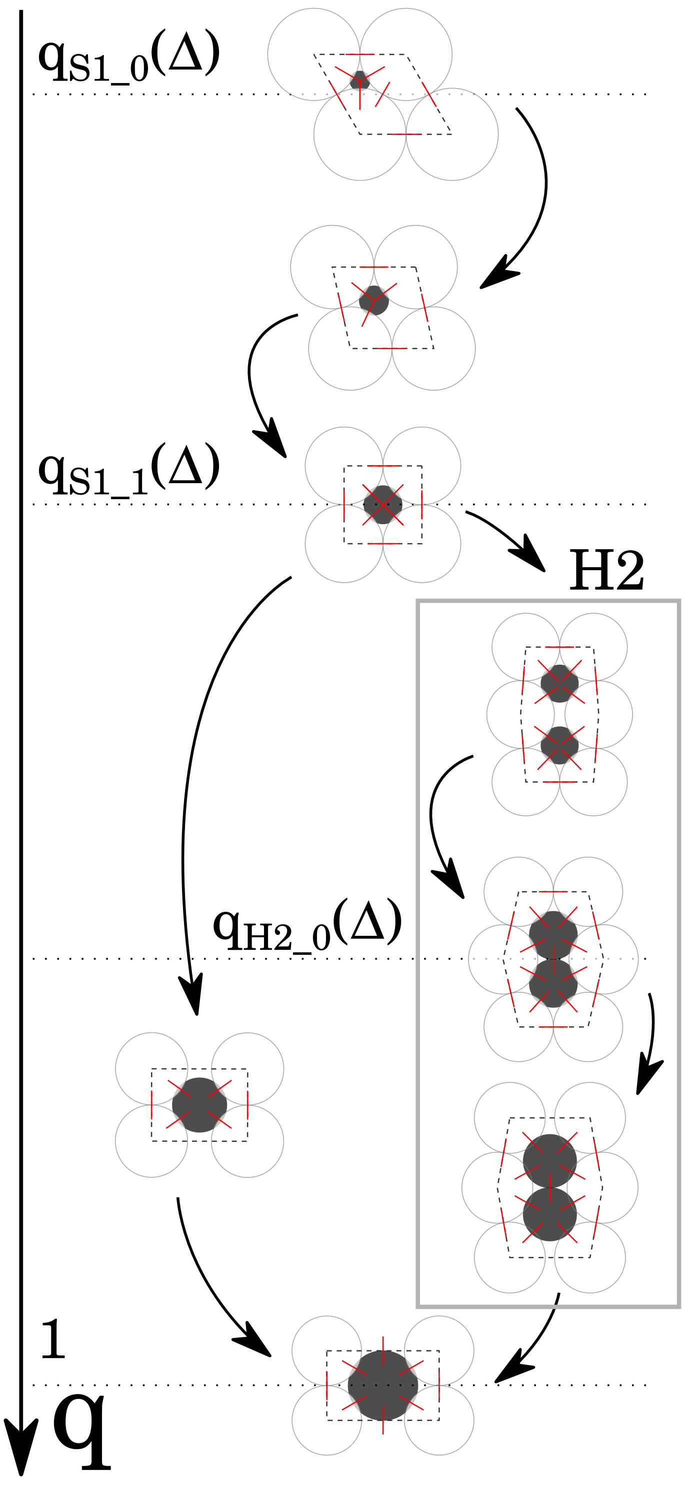


FIG. 5. Deformation paths of S1 and H2 structures. We label H2 the branch deforms the unit cell beyond $q_{S1\_1}(\Delta)$ by breaking one contact between large disks. The rest of the path is labeled S1.

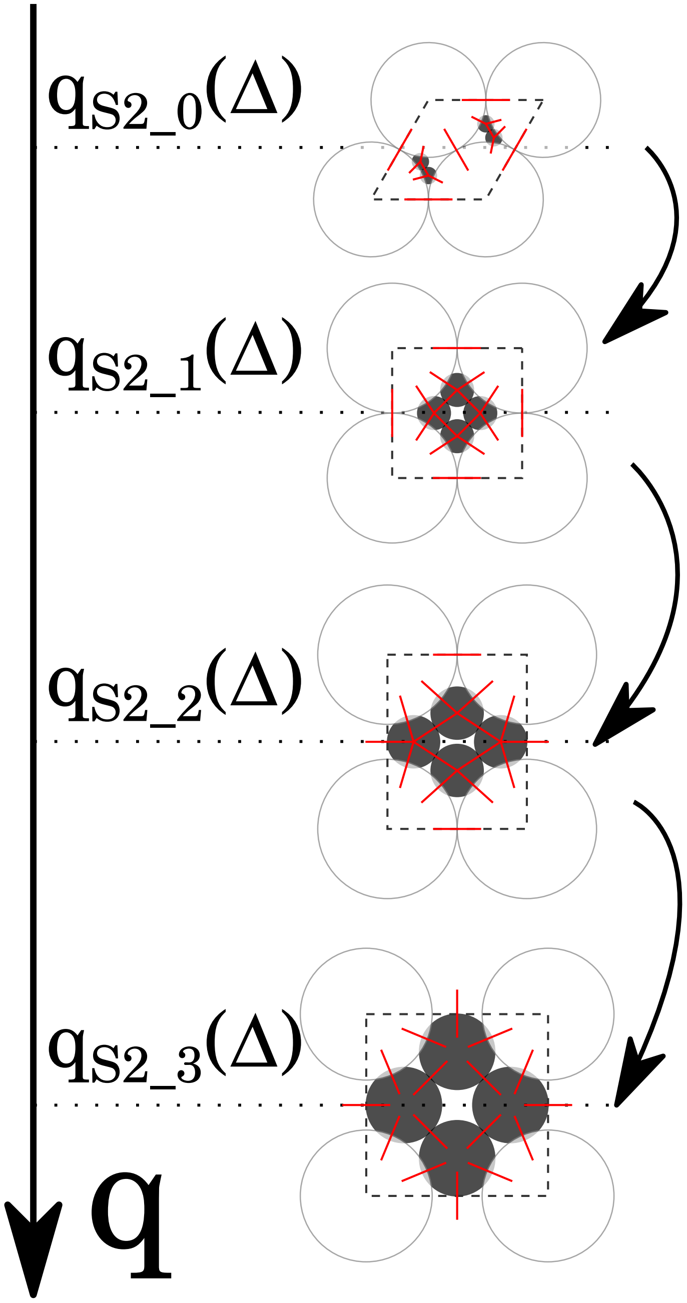


FIG. 6. S2 deformation path.

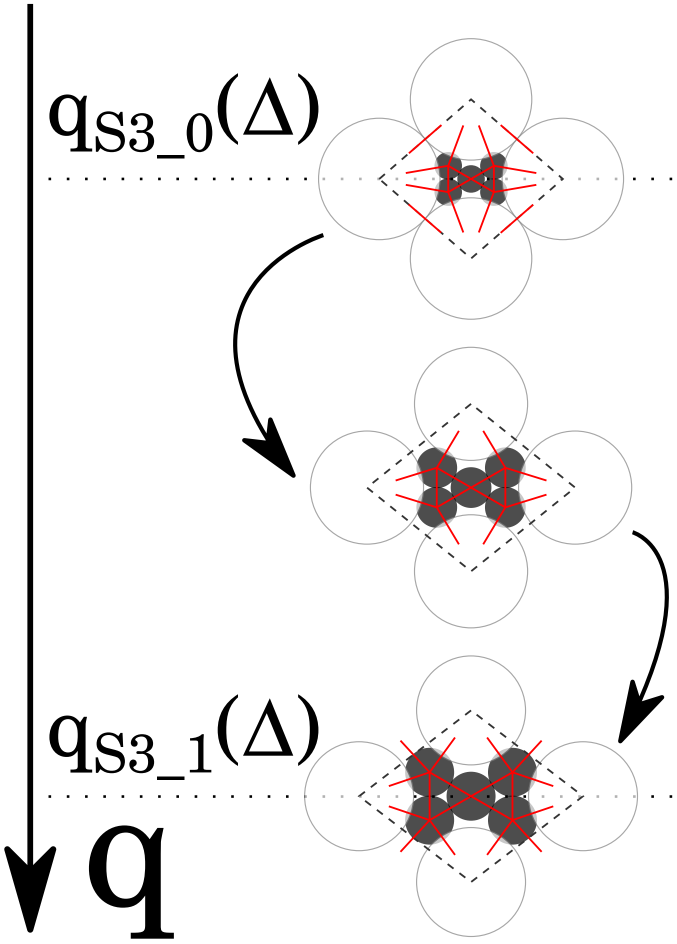


FIG. 7. S3 deformation path.

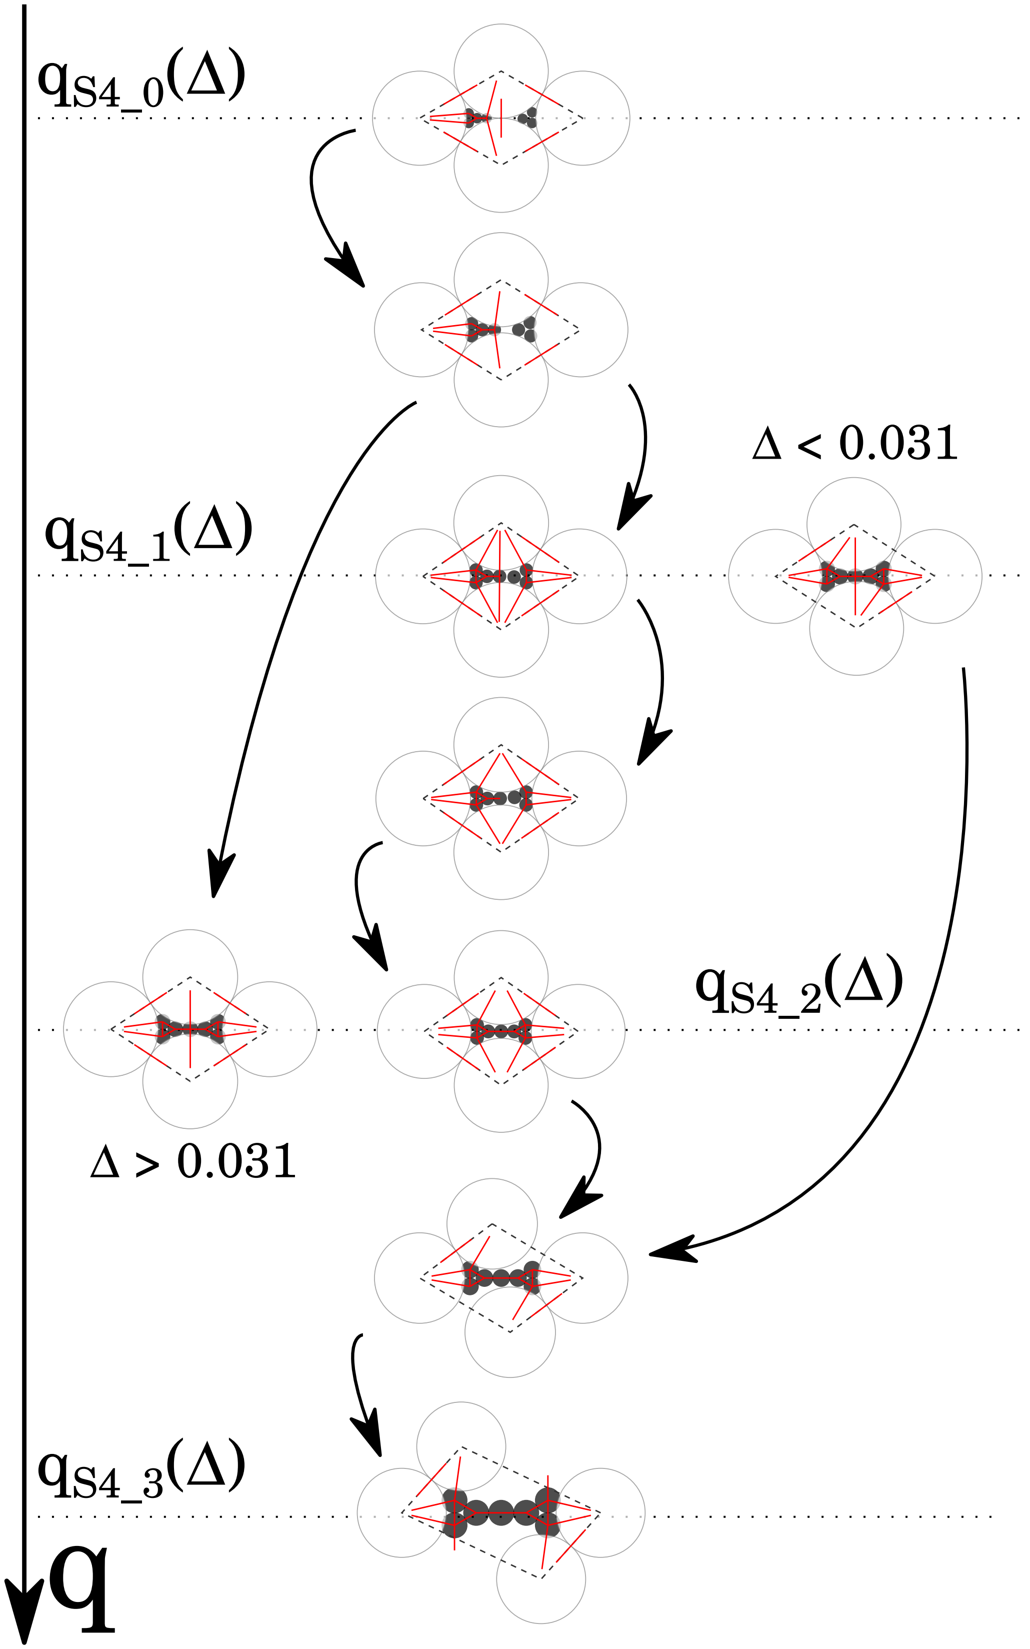


FIG. 8. S4 deformation path. Depending on the non-additivity parameter $\Delta$, different contacts occur first as the small disks are inflated, leading to two possible deformation branches. On the left branch ($\Delta > 0.031$), we could not find a deformation linking the S4 structure at $q_{S4\_3(\Delta)}$ and $q_{S4\_1(\Delta)}$

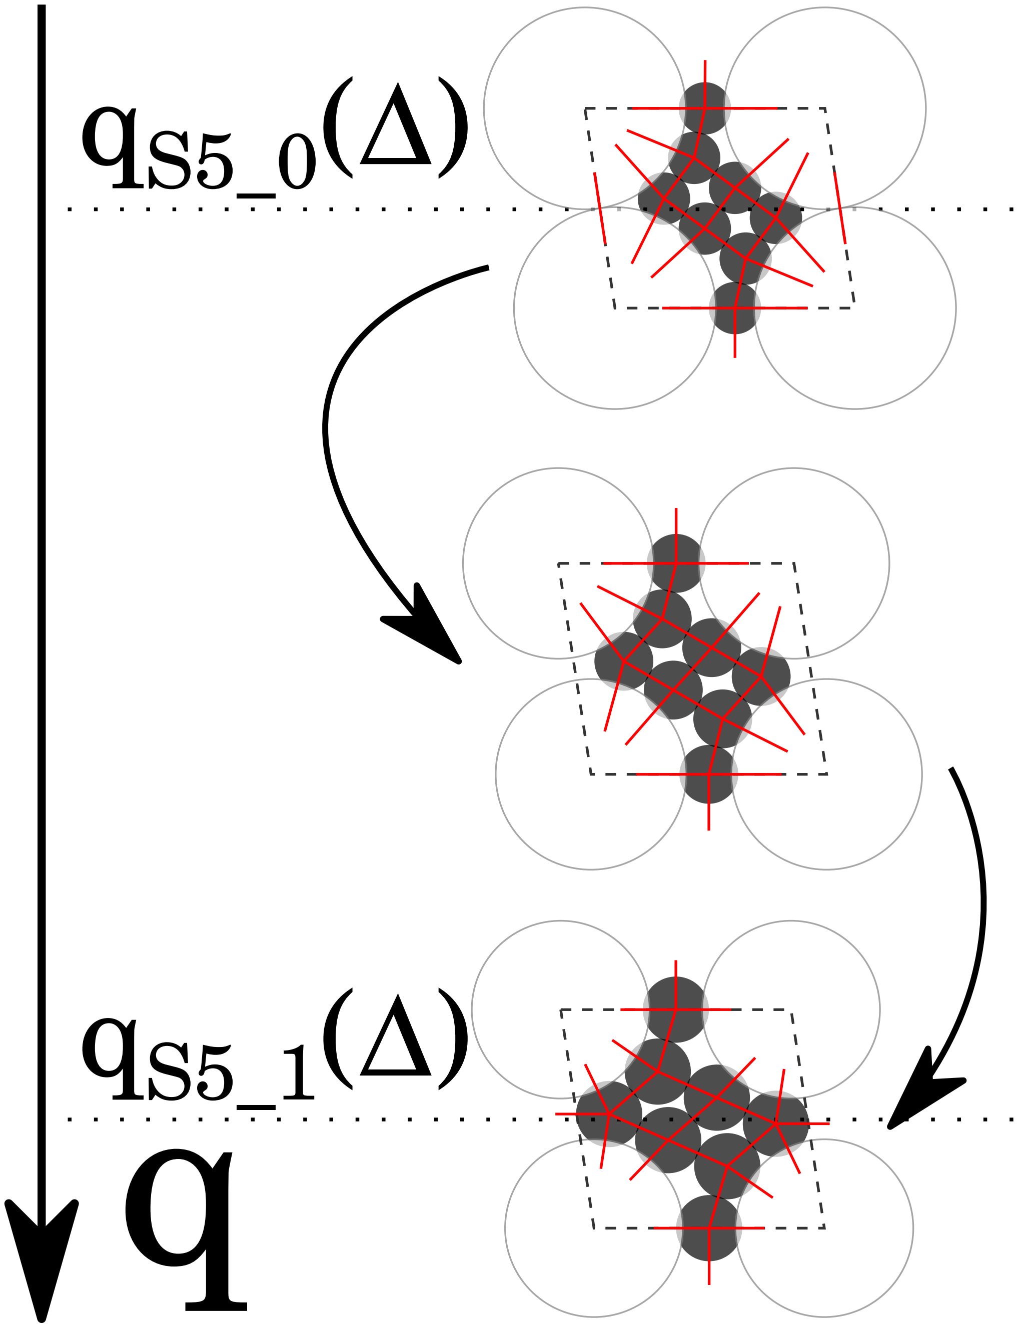


FIG. 9. S5 deformation path.

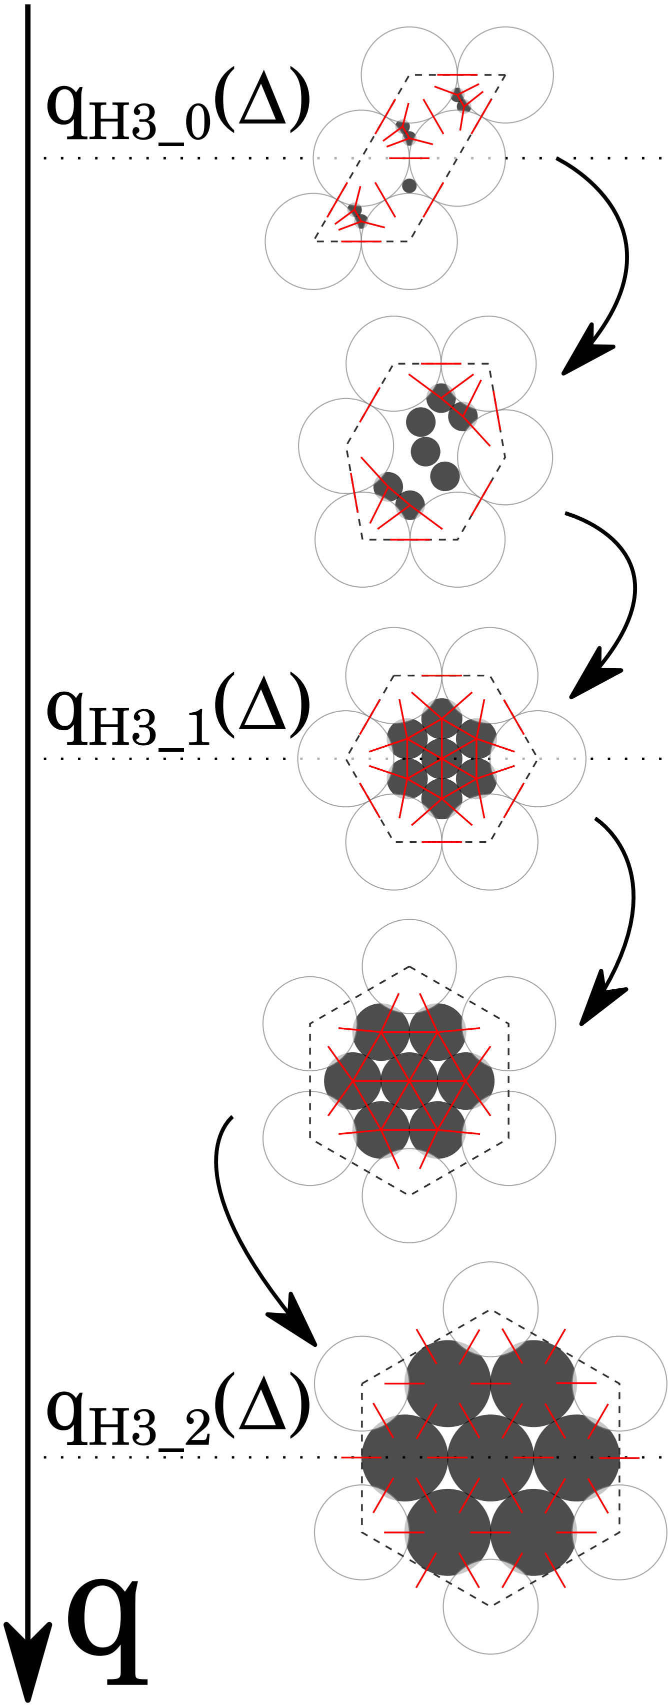


FIG. 10. H3 deformation path.

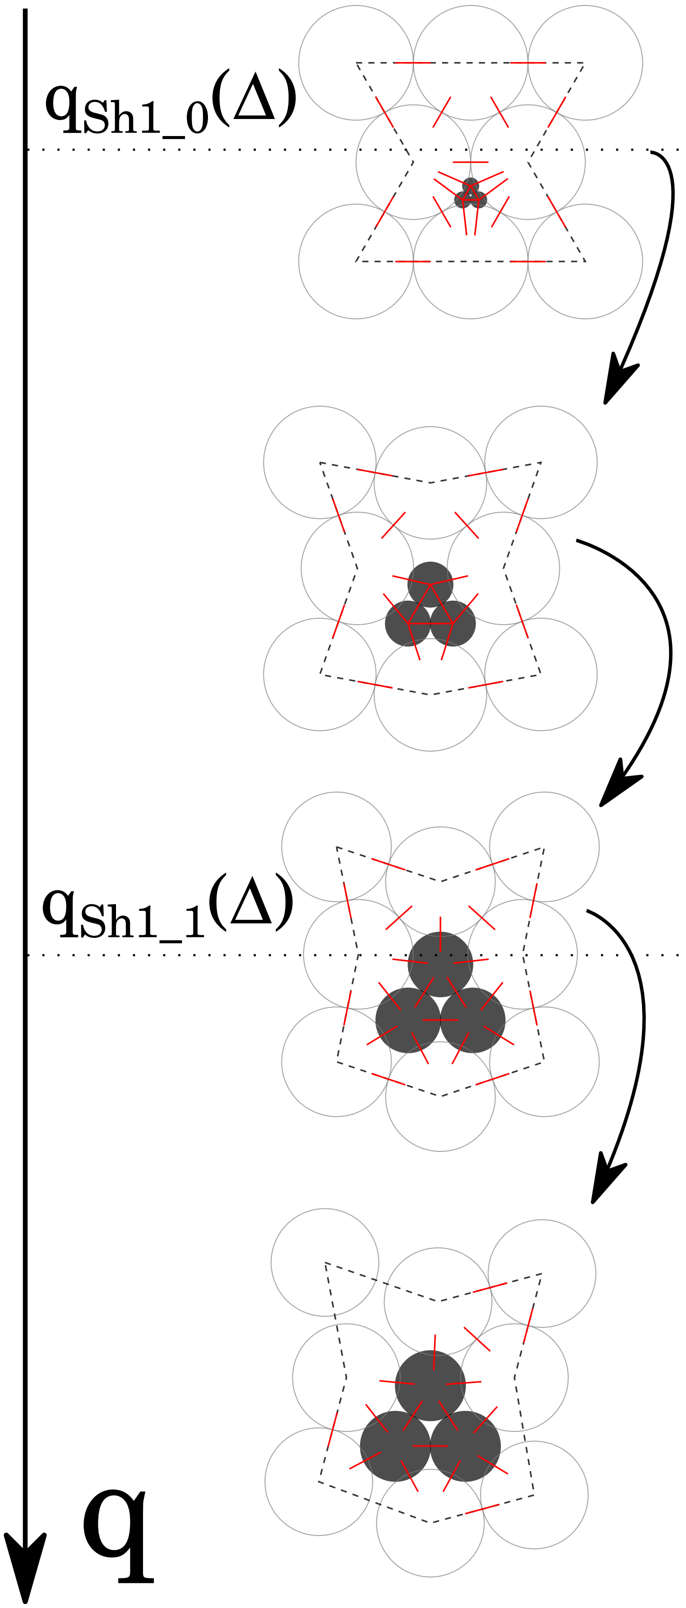


FIG. 11. Sh1 deformation path.

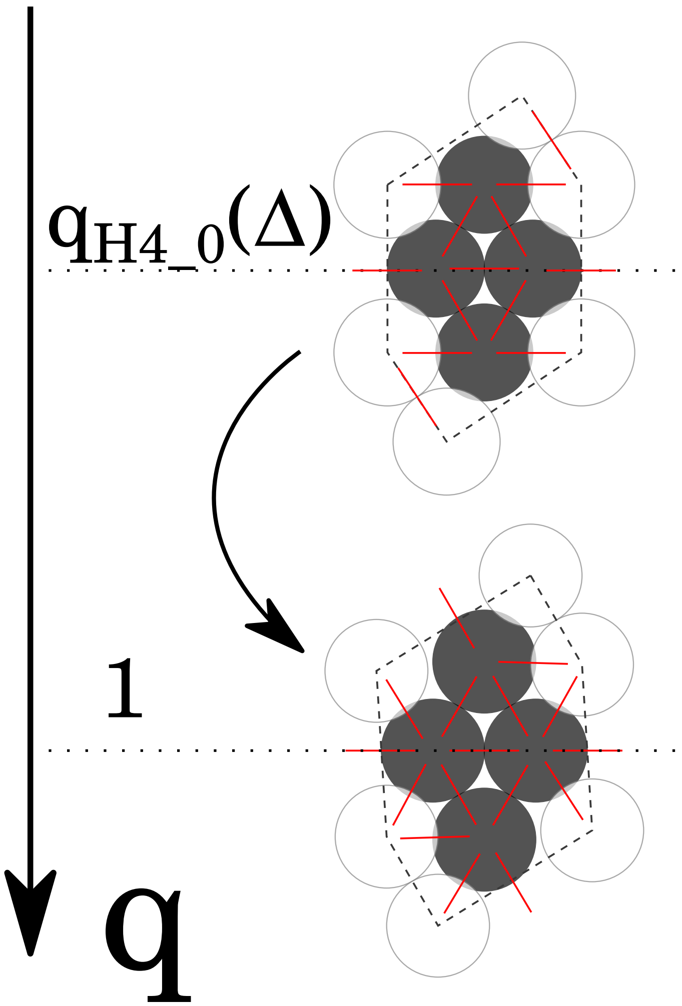


FIG. 12. H4 deformation path.

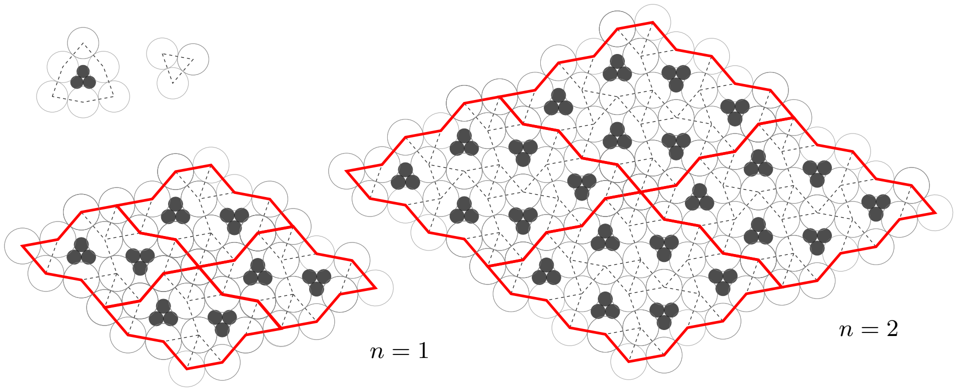


FIG. 13. The two first iterations of an (infinite) family of periodic structures with shield and triangular tiles (upper-left). They have the same volume per particle as the coexistence of Sh1 and $\mathrm{Hex_L}$ at the same fraction of small disks $p$.

[1] L. Filion, M. Marechal, B. van Oorschot, D. Pelt, F. Smallenburg, and M. Dijkstra, Phys. Rev. Lett. **103**, 188302 (2009).
[2] C. N. Likos and C. L. Henley, Phil. Mag. B **68**, 85 (1993).
[3] T. Fernique, A. Hashemi, and O. Sizova, in *Discrete Geometry for Computer Imagery*, Vol. 11414, edited by M. Couprie, J. Cousty, Y. Kenmochi, and N. Mustafa (Springer International Publishing, Cham, 2019) pp. 420–431.
[4] A. Meurer, C. P. Smith, M. Paprocki, O. Čertík, S. B. Kirpichev, M. Rocklin, A. Kumar, S. Ivanov, J. K. Moore, S. Singh, T. Rathnayake, S. Vig, B. E. Granger, R. P. Muller, F. Bonazzi, H. Gupta, S. Vats, F. Johansson, F. Pedregosa, M. J. Curry, A. R. Terrel, v. Roučka, A. Saboo, I. Fernando, S. Kulal, R. Cimrman, and A. Scopatz, PeerJ Comput. Sci. **3**, e103 (2017).

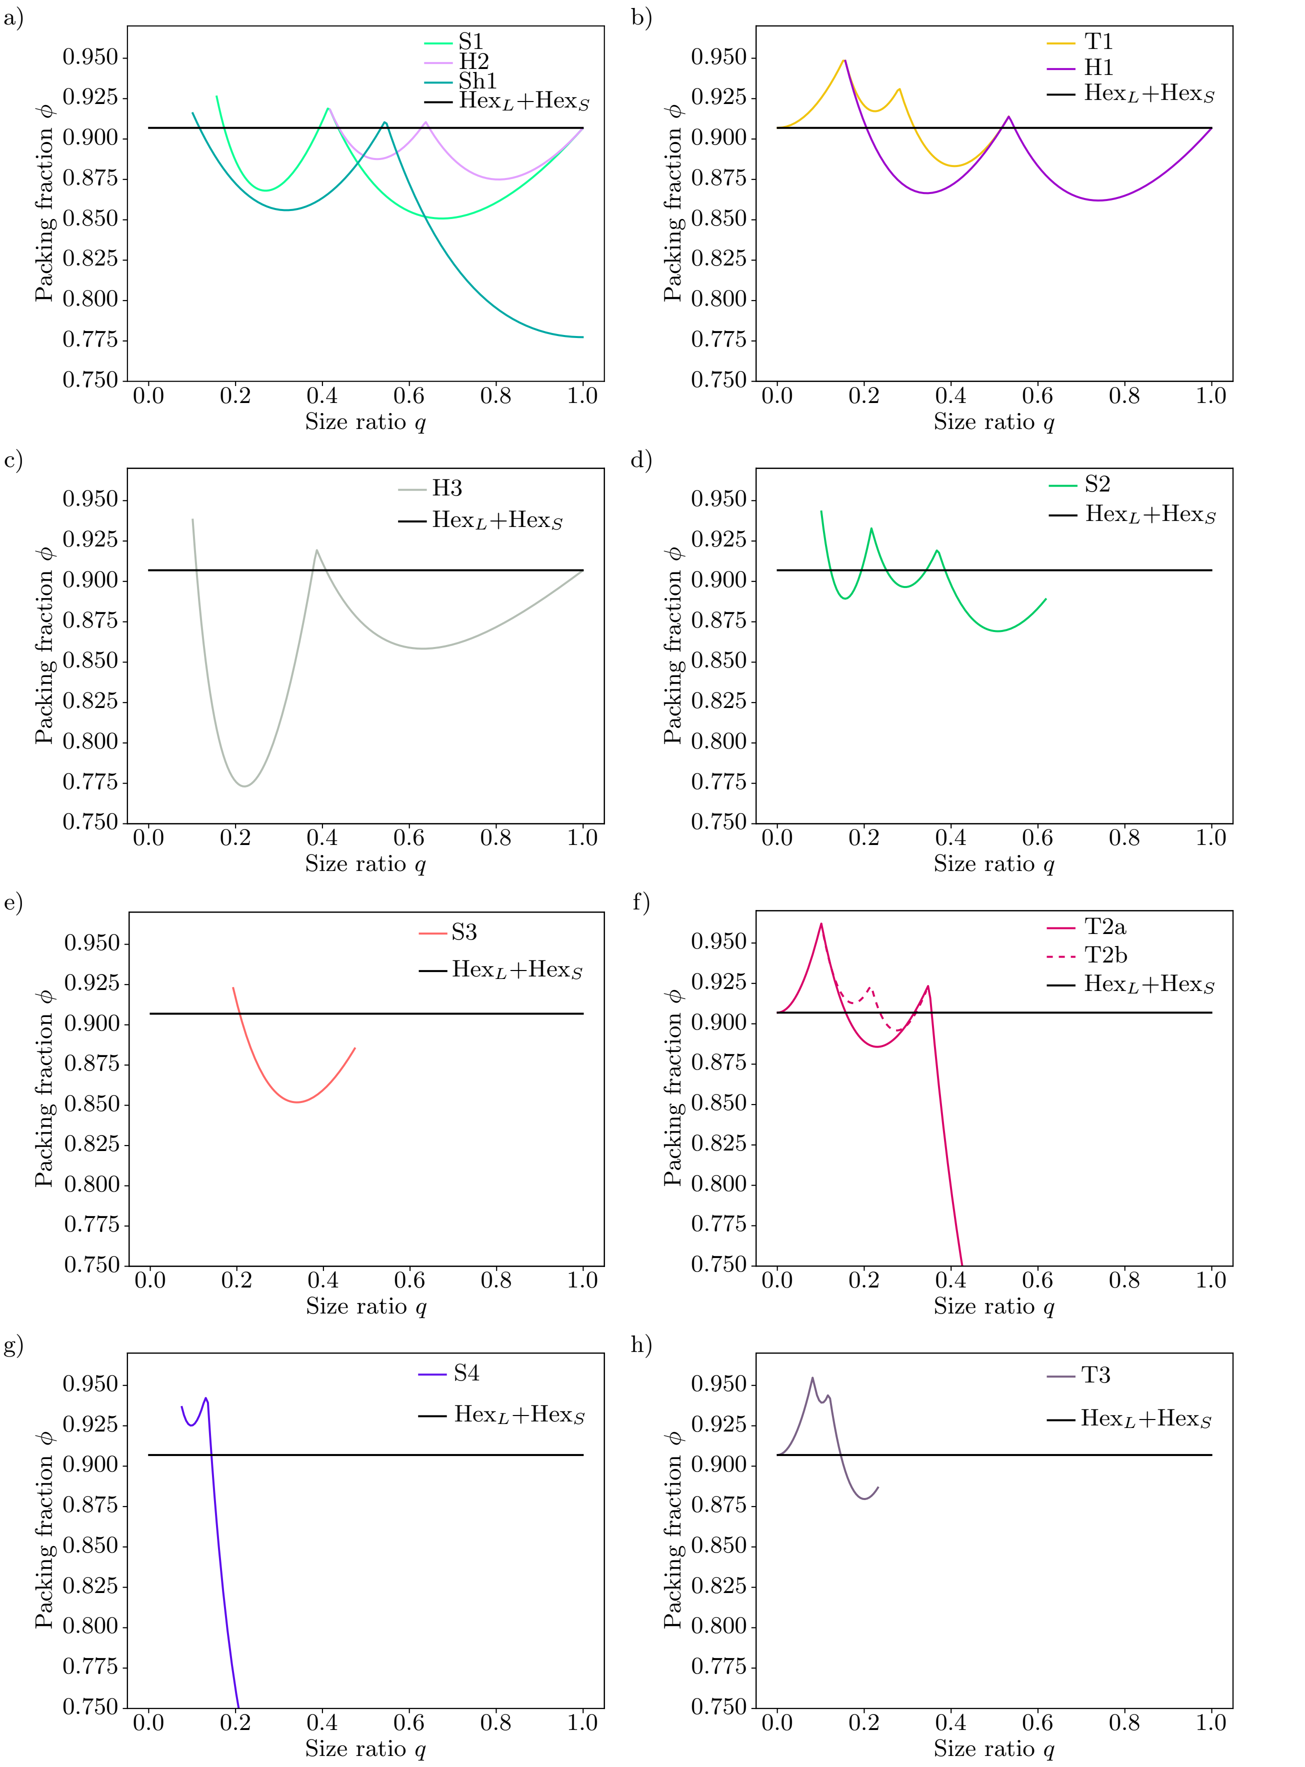


FIG. 14. Packing fraction of the pure phases at $\Delta = 0$, for compositions a) $x_S = 1/2$, b) 2/3, c) 7/9, d) 4/5, e) 5/6, f) 6/7, g) 7/8, and h) 8/9.
